# Supplementary material for: RedPen: Region- and Reason-Annotated Dataset of Unnatural Speech
Source: arXiv:2210.14406 source file (2022-10-26)
Supplement: Supplementary file 1 [file 99_appendix.tex]

\begin{figure*}[tb]
    \centering
    \includegraphics[width=.9\textwidth]{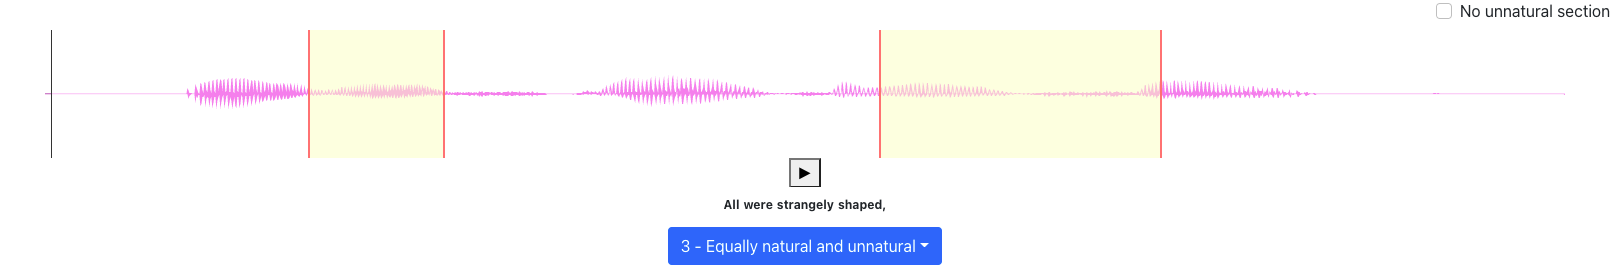}
    \caption{Region annotation sample.}
    \label{fig:redpen_sample}
\end{figure*}

\section{Human Annotation Details}
\label{sec:annotation_details}
In this section, we describe details of human annotation in section~\ref{sec:data_collection}.
For the first step of the data collection, we developed a new annotation tool collecting annotation of unnatural regions. Figure~\ref{fig:redpen_sample} shows the outline of our annotation tool. One of the main problem to develop the annotation tool is the gap between people's thought and the data format. People usually perceive speech data in unit of word which is discrete data, but the audio is nearly continuous which normally consists of 10000+ frames in a second. Considering this gap, our annotation tool basically annotate each region by word, but it also supports adjusting and creating continuous region onto audio waveform with dragging. 

Our main goal is to obtain annotations for unnatural speeches, but naturally synthesized speeches cannot be ignored because naturally synthesized speeches may have different type of errors. Considering our goal, we sampled 180 speeches from entire synthesis results in two steps. For the first step, we randomly sampled 45 speeches in all synthesized speeches, regardless of the audio quality. Next, we sampled 135 synthesized speeches in the audios whose MOS score $\leq$ 3. Consequently, our data can meet both large amount and various styles of unnaturalness annotations. 

When collecting the unnaturalness annotations, we used Amazon Mechanical Turk\footnote{\url{https://mturk.com}} as a crowdsourcing platform and own annotation tool for actual annotation. We hired 60 participants through Amazon Mechanical Turk. 
Each participant annotated 10 speeches, and three people participated in annotating each speech.
Each participants are paid above minimum wage. Considering evaluation of 10 speech samples take 20 minutes in average, we paid \$2.42 (1/3 of US federal minimum wage \$7.25).

In order to filter low-quality annotations, a human-recorded speech is included in 10 speeches. We excluded annotators who annotated to those human-recorded speeches, assuming the human-recorded speeches are completely natural. We also asked annotators to score the overall naturalness score as existing models evaluate. We collect these overall score to observe each person's perception relationship between traditional method and region annotations.

Our annotation work is reviewed and approved by the Institutional Review Board.

\section{Error Type Co-occurrence}
\label{app:cooccur_explain}
\begin{figure}[t]
    \centering
    \small
    \includegraphics[width=.499\textwidth,trim={0.5cm 0.1cm 0.1cm 0},clip]{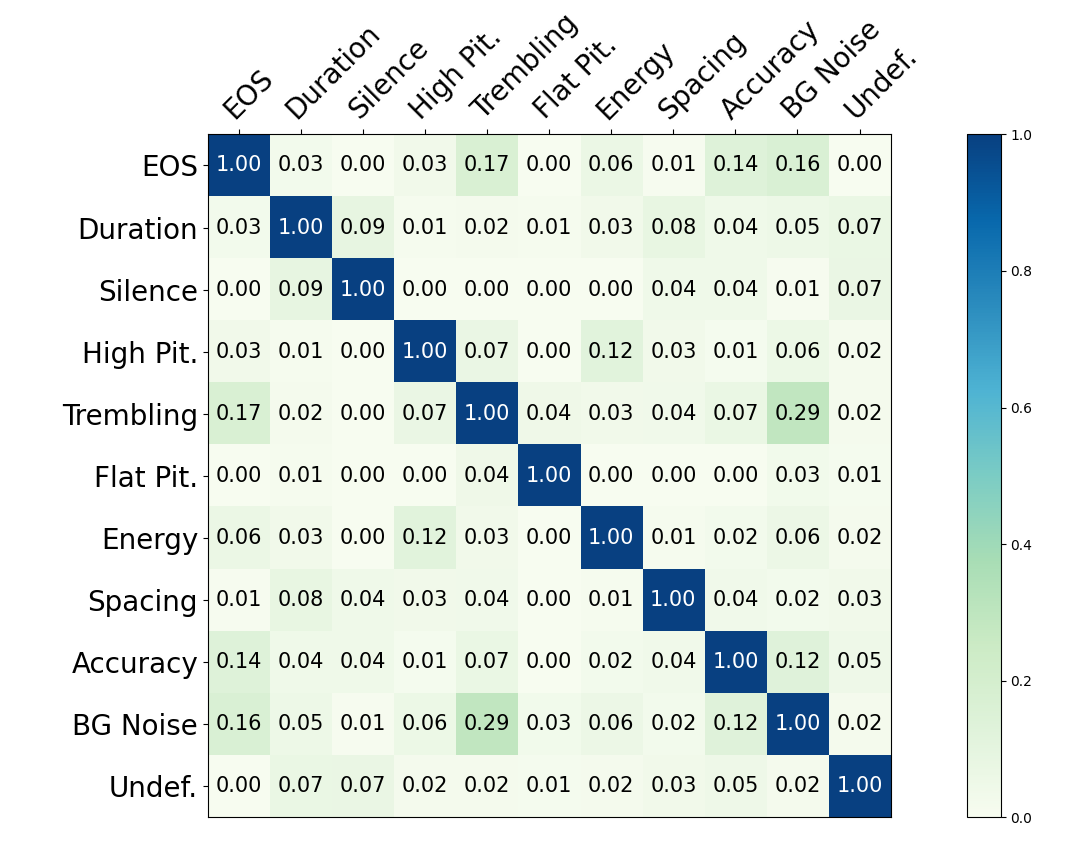}
    \caption{Co-ocurrence matrix between error types. Lighter block indicates higher co-occurrence of two error types.}
    \label{fig:cooccurrence}
\end{figure}

We assume that error types we defined should be independent on each other.
In fact, however, some unnatural regions may include multiple error types together such as having a background noise with high pitch and trembling voices.
% In order to cover as diverse errors as possible, error types should not overlap each other. %and undefined error should be minimized.
To measure the relationship between errors, we show the co-occurence matrix of error types in samples in RedPen. Co-occurrence score is computed as $\frac{\texttt{\# regions with both labels}}{\texttt{\# regions with one of two labels}}$. 
We assume that each type of error occurs once in a region, regardless of the size of the region. %Even though an error occurred at a temporary point, people may perceive surrounding region unnatural. 

As shown in Figure~\ref{fig:cooccurrence},  most error pairs have co-occurrence < 0.1, which indicates that there is no frequent overlap between two error types. 

However, there are some co-occurring cases over 0.1 even though any co-occurrence records below 0.3. 
End of speech error occurs with trembling, accuracy, and background noise error frequently. This co-occurrence would be from limitation of sequence-to-sequence speech synthesis model which have low prediction performance in long sequence \citep{ren2019fastspeech, hwang2021document}. Co-occurrence between high pitch and energy-related is based on high statistical correlation between pitch and energy \citep{hirschberg2006correlation}. Trembling and background noise have the most shared regions, because both errors are from noise problem. Trembling can be regarded as noise in voice, therefore the reason of two errors could be similar.

\section{Human-Model Correlation}
\label{app:model_correlation}
To observe the relevance between interpretation of MOS prediction model and human annotation, we compute Pearson's correlation between model interpretation and human annotations (bin annotation) for each error type and overall regions. 

\input{supplementary/model_human_correlation}

Table~\ref{tab:model_human_corr} describes correlation between model interpretation and annotated regions for each error type and overall human annotation. The correlation value is near 0 for all error types and overall, which indicates that model interpretation is irrelevant to any of the error types.
