# Supplementary material for: RedPen: Region- and Reason-Annotated Dataset of Unnatural Speech
Source: arXiv:2210.14406 source file (2022-10-26)
Supplement: Supplementary file 2 [file coocurrence.tex]

\begin{figure}[t]
    \centering
    \small
    \includegraphics[width=.499\textwidth,trim={0.5cm 0.1cm 0.1cm 0},clip]{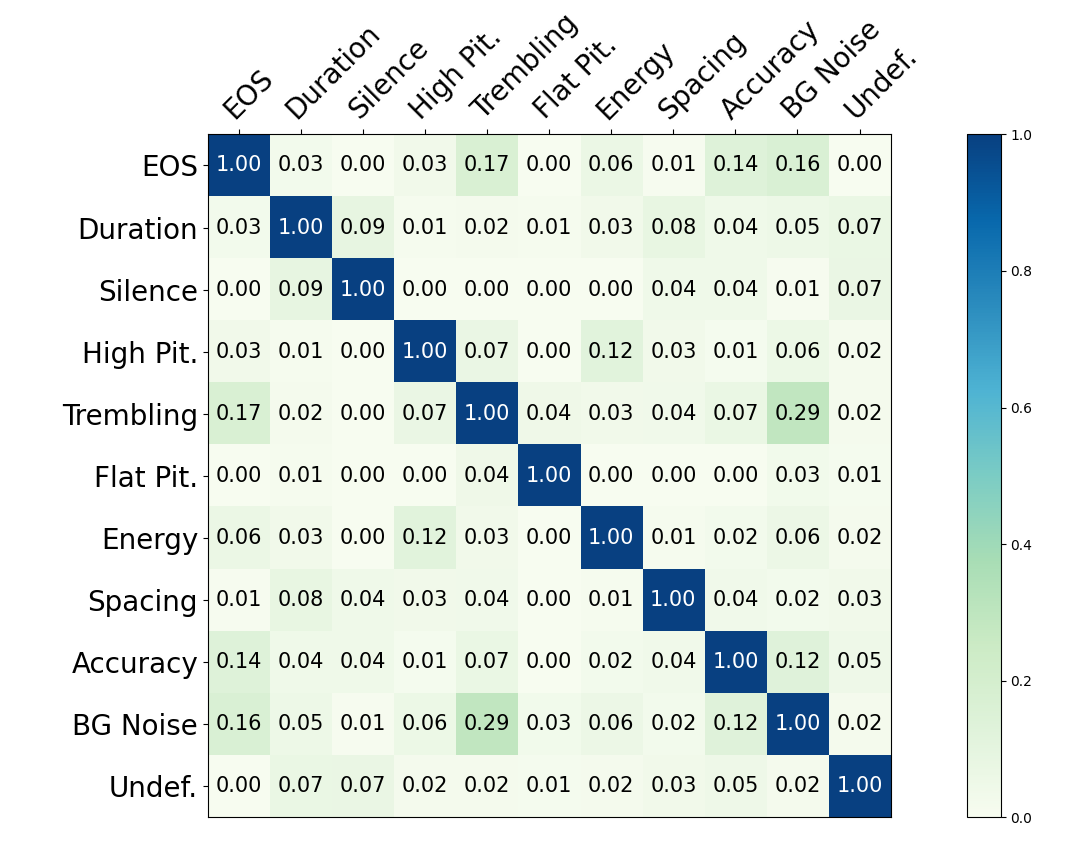}
    \caption{Co-ocurrence matrix between error types. Lighter block indicates higher co-occurrence of two error types.}
    \label{fig:cooccurrence}
\end{figure}
