# Supplementary material for: RedPen: Region- and Reason-Annotated Dataset of Unnatural Speech
Source: arXiv:2210.14406 source file (2022-10-26)
Supplement: Supplementary file 3 [file redpen_tool_sample.tex]

\begin{figure*}[tb]
    \centering
    \includegraphics[width=.9\textwidth]{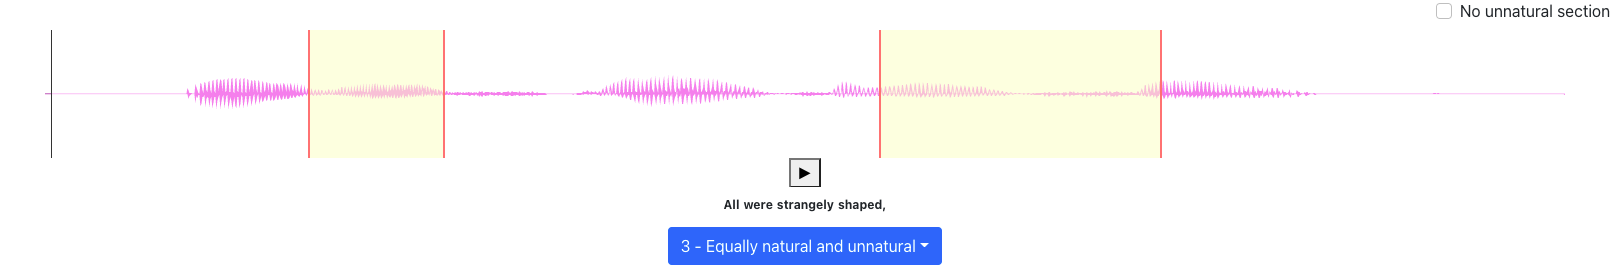}
    \caption{Region annotation sample.}
    \label{fig:redpen_sample}
\end{figure*}
